# Supplementary material for: On the use of Silver Standard Data for Zero-shot Classification Tasks in Information Extraction
Source: arXiv:2402.18061 source file (2024-03-06)
Supplement: Supplementary file 1 [file appendix.tex]

\section{Clean Data Detection Components}
This section presents how we adapt three noisy labels training algorithms, i.e., NLNL, O2U and DivideMix, to clean data detection modules. These modules use the same classifier, as shown in \ref{appendix:classifier}.
\label{appendix:o2u_dividemix_cddc}
\subsection{Negative Learning (NL) Method}
\label{appendix:nll}
In NL, the complementary label is randomly selected from the label space excluding the input label (possibly noisy). As shown in Eq.\ref{eq:loss_func}, the negative learning loss provides the model with the complementary label(s), telling what is incorrect and optimizing the output probability corresponding to the complementary label to be close to zero.

% \deleted[comment={}]{
% The negative learning loss function is shown as follows,
% \begin{equation}
%     \label{eq:loss_func}
%      \mathcal{L}_{neg}(f,\widehat{\y})=-\sum_{k=1}^{|\YM|} \widehat{\y}_k \log (1-\p_{k}),
% \end{equation}
% where $f$ is a classifier, $|\YM|$ is the number of relation types, $\widehat{\y}$ is a one-hot vector with the complementary label being one, $\widehat{\y}_k$ is the $k$-th element of $\widehat{\y}$, $\p$ is the output probability, and $\p_{k}$ is the $k$-th element of $\widehat{\p}$.
% }

The whole clean data detection process by using NL is presented in Algorithm \ref{alg:NL}. In our experiment, $n_{c}$ is equaled to the number of relation types.

\begin{algorithm}[t]
    \caption{Clean Data Detection using \textbf{NL}}
    \label{alg:NL}
    \begin{flushleft}
        \textbf{Input:} silver data $D_{silver}$ , total epoch $T$, number of complementary labels $n_c$. \\
    \end{flushleft}
    \begin{algorithmic}[1]
    % \FOR{$t$ in range $\textbf{T}$}
    \FOR{$t \gets 1 \ \TO \ $T}
        % \STATE Fetch batch from  $D_{silver}$.
        \STATE Generate $n_r$ complementary labels for each input label.
        \STATE Minimize Eq. \ref{eq:loss_func}.

        \STATE Calculate the confidence score of each sample in $D_{silver}$.
    \ENDFOR
    % \STATE  ${D}_{clean} = {\arg\max}_{D_s:\mid D_s \mid = \eta \cdot \mid D_{silver} \mid} \SM(D_s).$
    \STATE  Obtain clean data set ${D}_{clean}$ by Eq. \ref{eq:select_NL}.
  \end{algorithmic}
  \begin{flushleft}
    \textbf{Ouput:} clean data set $D_{clean}$.
  \end{flushleft}
\end{algorithm}
\subsection{Clean label detection by Overfitting to Underfitting (O2U)}
O2U \cite{huang2019o2u} exploited the loss of each sample to detect clean data in a special setting where the status of the model transfers from overfitting to underfitting cyclically. 
The status change is implemented by changing the learning rate cyclically. 
The intuition of O2U is the memorization effect \cite{arpit2017closer} which is stated as although deep networks can memorize noise data, they tend to learn simple patterns first. 
The clean samples can be quickly learned by deep networks, hence their losses maintain small once they are learned. 
Clean samples tend to have smaller losses in the whole training procedure. 
The hard samples and noisy samples are not memorized until it reaches the overfitting stage, hence their losses are large at the underfitting stage. 
Hence, by transferring the status from underfitting to overfitting and collecting the statistics of losses, it is possible to detect clean data.
In O2U-based clean data detection module, a classifier (see Appendix \ref{appendix:classifier} ) is trained in two phases, i.e., pretraining and cyclical training.

\paragraph{\textbf{Pretraining.}}
The network is pre-trained on the silver standard data with a constant learning rate. 
\paragraph{\textbf{Cyclical Training.}}
A cyclical learning rate is applied to train the classifier. During this process, the learning rate is changed from maximum to minimum repeatedly. 
In a training epoch, suppose the maximum learning rate is $r_{max}$ and the minimum learning rate is $r_{min}$, 
a linear learning rate decrease function $r(t)$ is adopted to adjust the learning rate as follows,

\begin{equation}
\begin{aligned}
r(t)=r_{max}-\frac{t}{E}\times(r_{max}-r_{min}),
\end{aligned}
\label{eq:o2u}
\end{equation} 

where $t$ is the $t$-th epoch of a cyclical training round, $E$ is the total number of epochs in each cyclical round, and $r(t)$ is the learning rate applied at epoch $t$ in a cyclical training round.

After training the classifier in the cyclical setting, we sort silver standard data by their summation losses of several rounds of underfitting to overfitting procedure. We select a fixed proportion $\eta$ of the silver data with smaller loss as clean data. 
Given that $\LM(D_s)$ is total loss of each sample in the selected data set $D_s$ , the clean data set $D_{clean}$ are selected as follows, 
\begin{equation}
\label{eq:select_O2U}
    {D}_{clean} = {\arg\min}_{D_s:\mid D_s \mid = \eta \cdot \mid D_{silver} \mid}\LM(D_s).
\end{equation}

\subsection{Clean label detection by \textbf{DivideMix}}
\label{sec:DivideMix}
DivideMix \cite{li2020dividemix} used a Gaussian Mixture Model to dynamically divide the noisy data into a labeled set with clean samples and an unlabeled set with noisy samples. DivideMix trained a classifier on the labeled set as well as unlabeled set in a semi-supervised manner. 
% The model will guess labels for the unlabeled set in the semi-supervised training.  
Two models are simultaneously trained for co-dividing and co-guessing to reduce confirmation bias. 
DivideMix can efficiently maintain small losses for clean samples but keep large losses for noisy samples.

When we apply DivideMix to clean data detection, we have modifications in generating data augmentation and applying MixMatch \cite{berthelot2019mixmatch} on the augmented labeled data and augmented unlabeled data. For data augmentation, we randomly replace the subject entity or object entity with other entities in the dataset with the same entity type. When applying MixMacth, DivideMix linearly interpolated inputs of random samples. 
However, text cannot be directly interpolated, while interpolation is straightforward for image pixels. 
Thus, as proposed by \cite{guo2019augmenting}, we interpolate the text embedding of random samples.

We use the cross-entropy loss to detect clean data. We select $D_{clean}$ using Eq. \ref{eq:select_O2U}

\section{Classifier}
\label{appendix:classifier}
We use the relation model in the PURE system \cite{zhong2020frustratingly} as the relation classifier. 
The input text is inserted with text markers to highlight the subject and object and their positions. 
Given a input text $x$, the subject span \textsc{Subject}, the object span \textsc{Object}, the subject entity type $t_{subj}$, and object entity type $t_{obj}$, 
Text markers are defined as $\langle \textsc{S:}t_{subj}\rangle$, $\langle \textsc{/S:}t_{subj}\rangle$, $\langle \textsc{O:}t_{obj}\rangle$, and $\langle \textsc{/O:}t_{obj}\rangle$. 
We insert them into the input text before and after the subject and object span. 
Let $\hat{x}$ denote the modified sentence with text markers inserted: 
\begin{align*}
    &\widehat{x} = \dots \langle \textsc{S:}e_{subj}\rangle \:\textsc{Subject}\:  \langle \textsc{/S:}e_{subj}\rangle \\
    &\dots \langle \textsc{O:}e_{obj}\rangle \:\textsc{Object}\:  \langle \textsc{/O:}e_{obj}\rangle \dots.
\end{align*}
% \begin{align*}
%     &\widehat{x} = \dots \langle \textsc{S:}e_i\rangle  \textsc{Subject} x_{\textsc{START}(i)} \dots, x_{\textsc{END}(i)} \langle \textsc{/S:}e_i\rangle \\
%     &\dots \langle \textsc{O:}e_j\rangle, x_{\textsc{START}(j)} \dots x_{\textsc{END}(j)} \langle \textsc{/O:}e_j\rangle \dots.
% \end{align*}

We concatenate the hidden state embeddings of the final layer in BERT \cite{devlin2018bert} at the subject start marker position and object start marker position as the contextual representations of $\hat{x}$,
\begin{equation*}
    \mathbf{h}_r(\hat{x})=[\mathbf{\widehat{x}}_{\widehat{\textsc{START}}_{subj}}; \mathbf{\widehat{x}}_{\widehat{\textsc{START}}_{obj}}],
\end{equation*}
where $\widehat{\textsc{START}}_{subj}$ and $\widehat{\textsc{START}}_{obj}$ are the position indices of $\langle \textsc{S:}e_{subj}\rangle$ and $\langle \textsc{O:}e_{obj}\rangle$ in $\hat{x}$, and $\mathbf{\widehat{x}}$ is a list of hidden state embeddings of all words in $\widehat{x}$.
Finally, the representation $\mathbf{h}_r(\hat{x})$ will be fed into a feedforward network to obtain the probability distribution of the relation type.

\begin{table}[tp]
    \centering
    \resizebox{0.45\textwidth}{!}{
        \begin{tabular}[H]{c c p{1cm}<{\centering} p{1cm}<{\centering} p{1.75cm}<{\centering}}
            \hline
           &  & Pr. & Rec. & F1 \\
          \hline\hline
          % precision,  recall, F1 
          \multirow{2}*{TACRED} 
          & TE classifier  & 63.54 &  42.39 & 52.33\small{$\pm 0.77$}\\
          & PURE classifier  & 55.81 & 55.25 & 64.33\small{$\pm 1.22$} \\
          \midrule
          \multirow{2}*{Wiki80} 
           & TE classifier & 53.88 & 45.08 & 45.08\small{$\pm 0.13$} \\
          & PURE classifier & 56.84 & 52.41 & 52.41\small{$\pm 0.14$}\\
          \hline
        \end{tabular}
    }
    \caption{The results of using different classifiers in our clean data detection module. }
    \label{tab:diff_classifier}
\end{table}

\revisejw{
As shown in table \ref{tab:diff_classifier}, PURE classifier outperform TE classifier on both TACRED and Wiki80 dataset. PURE classifier classifies data into N kinds of relation types while TE classifier classifies data into only three types: entailment, neutral, contradict and choose type with max entailment score as classified type. 
Negative learning is more suitable for multi-class classifier with more label types because more labels mean less probability to assign negative sample gold label and make negative learning more robust. 
}

% \revisety{TODO}Put it to Appendix: In the clean label detection process, the data used is only noisy training data, no dev data is needed. In order to save the time of clean label detection, we control the total number of epochs to be 10. For O2U, the epochs of pre-training and cyclical training are five, respectively. For NL, the total epochs negative learning process are ten. In the process of clean label detection, we select $\eta \times N_{train}$ clean samples, where $N_{train}$ is the number of training set of TACRED or Wiki80. For TACRED, we use datas that have positive pseudo labels to detect clean labels.

\section{Premise-Hypothesis Pairs Construction}
\label{appendix:p_h_pairs_constrcut}
We have different generation strategies when generating premise-hypothesis pairs for the positive relation and the negative relation. 

\begin{enumerate}
    \item \textbf{Positive Relation.} The positive relation means there is a relation between subject and object. For the positive relation, a \textbf{contradiction} hypothesis is generated using \texttt{no\_relation} verbalization template ``{\{subj\} and \{obj\} are not related}'', a \textbf{neutral} hypothesis is generated by randomly select a template that does not describe the ground truth relation, and a \textbf{entailment} hypothesis is generated with the templates that describes the ground truth relation.

    \item \textbf{Negative Relation.} The negative relation means subject and object are not related.  For the negative relation, a \textbf{contradiction} hypothesis is generated using has-relation template \texttt{There is a relation between  \{subj\} and \{obj\} }, a \textbf{neutral} hypothesis is generated by randomly select a positive relation template, and a \textbf{entailment} hypothesis is generated by the \texttt{no-relation} verbalization template mentioned above.
    
\end{enumerate}

\section{Experiments}

\subsection{Dataset Statistics}
\label{appendix:dataset}
The dataset statistics are shown in Table \ref{tab:statistics}.
TACRED consists of 42 relation labels including \texttt{no\_relation} and its relation distribution is skewed. 
TACRED provides entity type information.
Wiki80 contains 80 relation labels and its relation distribution is uniform. 
Since the test set of Wiki80 is not provided, we used the development set for testing. We take 20\% of the training data as the development set.

The noise ratios of silver standard data are 16.67\% and 58.88\% on TACRED and Wiki80 respectively. 
In TACRED, \texttt{no\_relation} is a major class, accounting for 85.75\% of whole data. We also provide the noise ratio of only positive relation data on TACRED, i.e., 42.01\%. 

The statistics of WikiFact are shown in Table \ref{tab:statistics}. 
We randomly select 45K instances from the whole WikiFact dataset as the extra data candidate pool as the whole dataset is very large. 
After applying different clean data detection algorithms, we finally select 800/1500 samples in WikiFact as extra data for TACRED/Wiki80 datasets.
% Here we use two kinds of dataset to test our method. For TACRED, the previous method often exclude the \textbf{no-relation} sample for better outcome. But we take it into consideration to make the experiment more convincing. 
% For wiki80, the initial dataset only provides the train(50400) and test(5600) set. And we spilt the train set and 80\% for training(40320) while 20\% for testing(10080). 
% Then for the entity type in wiki80, we use \textbf{MLM} to attach some type to each entity.
\begin{table}[H]
    \centering
    \resizebox{0.5\textwidth}{!}{
        \begin{tabular}[H]{ccccccc}
            \hline

          \multirow{2}{*}{ Dataset} & \multirow{2}*{Relation Types} & \multirow{2}*{Entity Types} & \multirow{2}*{Distribution} & \multicolumn{3}{c}{Instances} \\ &&&&Train & Dev & Test \\
          
          \hline
          
          TACRED & 42 & 17 & Skewed & 68124 & 22631 & 15509 \\
          Wiki80 & 80 & 29 & Uniform & 40320 & 10080 & 5600 \\ 
          WikiFact & 923 & 126 & Skewed & 2236367 & 276967 & 279699 \\ 
          
          \hline

        \end{tabular}
    }
    \caption{The statistics of TACRED and Wiki80 datasets. Each instance is a sentence with two entities and their entity types.}
    \label{tab:statistics}
\end{table}

\subsection{Entity Types Generation}
\label{appendix:generate_entity_type}
To obtain entity types in Wiki80, we finetune a pretrained language model \cite{devlin2018bert} using prompt learning paradigm on DBpedia dataset \cite{bizer2009dbpedia} to predict the entity type. 
The prompt template is designed as ``\{entity\} is a \texttt{[MASK]}''. 
DBpedia describes more than 2.6 million entities. Each text describes one entity and has a class label. 
We treat the class label as the entity type. 
At the inference phase, the prediction for the \texttt{[MASK]} token is used as the entity type for the entity on Wiki80.

\subsection{Compared Methods}
\label{appendix:compared_methods}
We briefly introduce baselines using different losses.

\textbf{CE} (Cross Entropy loss) has been widely used as optimization loss. We consider it as a baseline.
% It aims to use cross-entropy loss to train a relation classifier using noisy label attached to train set to classify relations.

\textbf{BSH} (Bootstrap Hard loss) \cite{reed2014training} consider neural network predictions are possible to be correct. 
BSH modified the CE loss and used a weighted combination of predicted and input labels (possibly noisy) as the correct labels. Hard labels are used as they have better performance. The hard label is the one-hot vector after taking $\argmax$ operation on the prediction distribution vector.
% BSH add a new component into CE loss like ($\y$ is one-hot ground truth vector and $\q$ is the prediction distribution): 
% \begin{equation}
%     BSL(\y,\d)= - \beta {\y}^{T} \log \q - (1-\beta) \z \log \q.
% \end{equation}
% By using the entropy of model prediction to measure the model confidence of predictions, we can avoid the overfitting. 
% Alternatively, 
% It replaces the cross-entropy loss with bootstrap hard loss which is one kind of noisy robust losses shown in \cite{reed2014training}.

\textbf{GCE} (Generalized Cross Entropy loss) \cite{zhang2018generalized} combined the CE loss and mean absolute error (MAE) loss via the negative Box-Cox transformation \cite{box1964analysis}. The MAE loss is proved to be noise-robust. 
% combined CE and mean absolute error (MAE) loss
% of the prediction distribution d:
% \begin{equation}
%     GCE(y,d)=\frac{1-y^{T}(d^{1-\beta})}{1-\beta}
% \end{equation}
% It combine the CE loss and MAE loss by controlling the value of $\beta$, which becomes MAE when $\beta$=0 and is equivalent to CE when $\beta$ approaches 1. So GCE can make the train process convergent fast like CE and noise robust like MAE.
% which is the negative Box-Cox transformation \cite{box1964analysis} of the predicted distribution d.

\textbf{SCE} (Symmetric Cross Entropy loss) \cite{wang2019symmetric} combined the CE loss and a noise-robust counterpart Reverse Cross Entropy (RCE) to deal with a weakness of CE.
CE tends to overfit noisy labels on ``easy'' classes and underfit on ``hard'' classes.
% can address both the hard class under learning and noisy label overfitting problems of CE.
% (CE) exhibits overfitting to noisy labels on some classes (“easy” classes), but more surprisingly, it also suffers from significant under learning on some other classes (“hard” classes).

% . SCE is like the BSH where it contains a non-noisy-robust loss part of CE and the other noisy-robust part of reverse cross entropy(RCE) in SCE like:
% \begin{equation}
%     SCE(y,d)=-\beta y^{T}logd-(1-\beta) d^{T}logy
% \end{equation}
% RCE defines log0 to be a negative constant A and is reduced to MAE when A= -2. SCE is shown to be noisy-robust for the existence of RCE.
% to train which includes a noise-robust part of RCE and non-noise-robust part of CE and has been shown robust to label noise \cite{wang2019symmetric}.
% CE by itself is not sufficient for learning of hard classes, especially under the noisy label scenario.

\textbf{ER-GCE} (Entropy Regularized Generalized Cross Entropy loss) \cite{jin2021instance} improved GCE by interpolating the CE loss with an entropy regularizer. It has a tighter bound than GCE. 
% \begin{equation}
%     ER-GCE(y,d)=\frac{\beta (1-y^{T}(d^{1-\beta}))}{1-\beta} +(1-\beta)H(d)
% \end{equation}
% \begin{align*}
%     ER-GCE(y,d)=&\frac{\beta (1-y^{T}(d^{1-\beta}))}{1-\beta} \\
%     &+(1-\beta)H(d)
% \end{align*}

%  ER-GCE is the further improvement of GCE by interpolating it with an entropy regularizer. Because both GCE and the entropy are bounded, the sum of both losses results in a noise-robust loss with tighter bounds than GCE by itself, making it more noise-robust.

\textbf{Co-Regularization} \cite{zhou2021learning} trained several classifiers with the same structures but different parameter initialization, and regularized all models to generate similar predictions rather than overfit the input (possibly noisy) labels. 
% The regularization minimizes the Kullback–Leibler (KL) divergence among predicted probability distributions by all classifier.  #zzq_save_sapce

\subsection{Full Constraints Comparison}
\label{appendix:full_constraint}
\revisejw{
We make some revisions to initial constraints defined in \textbf{LaVeEntail} for information leaking. Such as, obj type of \texttt{org:website} is restricted to only \texttt{URL} type in intial \textbf{LaVeEntail} definition. But many other website is recognized as \texttt{NUMBER} (0.0.0.0 is ip\_addr) and we extend full relation constraints in \textbf{LaVeEntail} to partial relation constraints allowing more reasonable obj type.
}

\revisejw{
Also, we compare our method with \textbf{LaVeEntail} under full constraints setting. As table \ref{tab:full_constraints} is shown, our method still outperform LaVeEntail given full constraints. Upper \textit{+} means full constraints and we directly use \textbf{LaVeEntail} results \cite{sainz2021label} marked with underlines. Under stricter type constraints, both methods obtain improvement compared to partial constraints results in table \ref{tab:main_result}. 
}

\begin{table}[htbp]
    \centering
    
    \resizebox{0.45\textwidth}{!}{
        \begin{tabular}[H]{c c p{1cm}<{\centering} p{1cm}<{\centering} p{1.75cm}<{\centering}}
             \hline
           &  & Pr. & Rec. & F1 \\
          \hline\hline
          \multirow{2}*{TACRED} 
          & $LaVeEntail^{+}$  & \underline{63.2} &  \underline{59.8} & \underline{61.4\small{$\pm 1.0$}}\\
           \cline{2-5}
          & $Our Method^{+}$  &  72.60 & 59.98 & 65.59\small{$\pm 1.62$} \\
          \midrule
        \end{tabular}
    }
    \caption{The results of using full constraints defined in LaVeEntail. }
    \label{tab:full_constraints}
\end{table}

\subsection{Dataset Samples}
\label{appendix:data_samples}
% \revisety{All of the methods in the third block are evaluated on class-balanced CV domain datasets, such as CIFAR-10 and CIFAR-100. However, TACRED has a long-tailed distribution, and Wiki80 is class-balanced, which explains such noisy label learning methods cannot outperform LaVeEntail in TACRED.}
As shown in Table \ref{tab:main_result}, In TACRED, the semi-supervised based methods still cannot outperform LaVeEntail. In Wiki80, the semi-supervised based methods except the self-training method can outperform or be comparable with LaVeEntail. 
The possible reason is that although the noise ratio of TACRED is lower than that of Wiki80, TACRED is a more challenging dataset than Wiki80. 
Table \ref{tab:wiki_samples} shows that the sentences in TACRED have a more complex context, while texts are straightforward in Wiki80. 
Also, TACRED has large intra-class differences compared with Wiki80. 
Table \ref{tab:wiki_samples_show_fix_structure} shows that instances in TACRED have large intra-class differences while instances in Wiki80 have similar structures.
For Wiki80, as long as these semi-supervised based methods can identify a few clean samples for each class, they can fully utilize the semi-supervised learning assumption \cite{chapelle2009semi} (i.e., points that are close to each other are more likely to share a label) to achieve good results. But in TACRED, data that share a label might be different in the input space.

\begin{table*}[h]

\centering
\resizebox{0.95\textwidth}{!}{
\begin{tabular}{|p{2cm}|p{9.5cm}|p{9.5cm}|}
	\hline
    \textbf{Relation}&\textbf{Instance in TACRED}&\textbf{Instance in Wiki80}\\
    
    %%%%%%%%%%%%%%%%%%%%%%%%%%%%%%%%%%%%%%%%%%%%%%%%%%%%%%%%%%%%%%%%%%%%%%%%%%5
    \hline \multirow{10}*{ religion} 
    & 
    Iran 's supreme leader \textcolor{red}{ Ayatollah Ali Khamenei } on Wednesday condemned Israel 's works near the flashpoint mosque compound in Jerusalem, urging \textcolor{blue}{ Muslim } countries to make the Jewish state regret the move.
    &
    \textcolor{red}{ Angelo Scola } ( born 7 November 1941 ) is an Italian Cardinal of the \textcolor{blue}{ Catholic Church } , philosopher and theologian.
    \\
    \cline{2-3}
    &
    Though not a household name, Wildmon has considerable clout; \textcolor{red}{ his } group has a vast mailing list and a proven ability to mobilize \textcolor{blue}{ Christian } conservatives by the hundreds of thousands.
    &
    \textcolor{red}{ Vincenzo Maria Sarnelli } ( 5 April 1835–7 January 1898 ) was an Italian \textcolor{blue}{ Catholic } archbishop.
    \\
    \cline{2-3}
    &
    \textcolor{red}{ Carson } 's grandmother raised him in a Baptist church and enrolled him at an inner-city \textcolor{blue}{ Catholic } school, where he entertained the idea of becoming a priest.
    &
    \textcolor{red}{ Giovanni Arcimboldi } ( died 1488 ) ( called the Cardinal of Novara or the Cardinal of Milan ) was an Italian \textcolor{blue}{ Roman Catholic } bishop and cardinal.
    \\
    \cline{2-3}
    &
    Chalabi, \textcolor{red}{ Mahdi } and Solagh all represent the Iraq National Alliance, the main \textcolor{blue}{ Shiite } religious list .
    &
    \textcolor{red}{ Vazgen I }, head of the \textcolor{blue}{ Armenian Apostolic Church }, sent Pope Paul VI a letter mourning Agagianian 's death.
    \\
    \cline{2-3}
    
    &
    Note: My thinking he is the worst has little to do with him being \textcolor{blue}{ Muslim }, since I think the other Muslim Congressman, \textcolor{red}{ Andre Carson } is a pretty good guy.
    &
    There are \textcolor{red}{ Sámi } Christians who believe in \textcolor{blue}{ Laestadianism } that use Ipmil for God.
    \\
    \cline{1-3}

\end{tabular}
}
\caption{Some instances on TACRED and Wiki80. The subject is marked in \textcolor{blue}{blue}, and the object is marked in \textcolor{red}{red}. }
\label{tab:wiki_samples}
\end{table*}

\begin{table*}[h]

\centering
\resizebox{0.95\textwidth}{!}{
\begin{tabular}{|p{9.5cm}|p{9.5cm}|}
	\hline
    Instances of "per:cities\_of\_residence" on \textbf{TACRED} & Instances of "taxon rank" on \textbf{Wiki80}\\
    
    %%%%%%%%%%%%%%%%%%%%%%%%%%%%%%%%%%%%%%%%%%%%%%%%%%%%%%%%%%%%%%%%%%%%%%%%%%5
    \hline 
    On the July morning in 1944 when \textcolor{red}{ she } boarded a Greyhound bus in \textcolor{blue}{ Gloucester } bound for Baltimore , Kirkaldy was not thinking about tackling racial segregation.
    &
    Culeolus is a genus of ascidian tunicates in the \textcolor{blue}{ family } \textcolor{red}{ Pyuridae }.
    \\
    \cline{1-2}
    She stayed at her home in \textcolor{blue}{ Wasilla }, located 40 miles to the north, but was expected in her office on Friday, spokesman \textcolor{red}{ Bill McAllister } said.
    &
    It is the only recognized extant genus in the \textcolor{blue}{ family } \textcolor{red}{ Equidae }.
    \\
    \cline{1-2}
    In \textcolor{blue}{ Vienna }, Austria, on Monday , International Atomic Energy Agency chief \textcolor{red}{ Mohamed ElBaradei } lamented a `` stalemate '' in efforts to begin talks over Iran 's nuclear program.
    &
    Polyozellus is a fungal genus in the \textcolor{blue}{ family } \textcolor{red}{ Thelephoraceae }, a grouping of mushrooms known collectively as the leathery earthfans.
    \\
    \cline{1-2}
    At her death , \textcolor{red}{ she } was assistant clinical professor emeritus of psychiatry at Albert Einstein College of Medicine of Yeshiva University in the \textcolor{blue}{ Bronx }.
    &
    Megalaria is a genus of lichenized fungi in the \textcolor{blue}{ family } \textcolor{red}{ Megalariaceae }.
    \\
    \cline{1-2}
    His death was confirmed by Hazel McCallion , mayor of \textcolor{blue}{ Mississauga } , Ontario , the Toronto suburb where \textcolor{red}{ Peterson } lived.
    &
    Leucothoe is a genus of amphipods in the \textcolor{blue}{ family } \textcolor{red}{ Leucothoidae }.
    \\
    \cline{1-2}

\end{tabular}
}
\caption{Some instance on TACRED and Wiki80. The subject is marked in \textcolor{blue}{blue}, and the object is marked in \textcolor{red}{red}.}
\label{tab:wiki_samples_show_fix_structure}
\end{table*}

\subsection{Clean Data Detection Module Analysis}
\label{appendix:histogram_clean_noisy}
We also plot the histogram of confidence scores or losses on silver standard data. As shown in the Figure \ref{fig:clean_noisy}, NLNL has a better ability to distinguish clean and noisy data. The clean and noisy data are well separated by confidence scores. 
% \revisety{Table \ref{tab:human_eval} shows that, compared with silver standard data, the clean data has high accuracy,zz  thus being worthy of finetuning pretrained model.}
\begin{table}[htbp]
    \centering
    \resizebox{0.3\textwidth}{!}{
        \begin{tabular}{c|cc}
            \toprule
            & Silver data & Clean data  \\
             
            \midrule
            \midrule
            TACRED & 57.50\% & 80.42\%   \\
            \midrule
            Wiki80 & 48.96\% & 89.42\%   \\
            \bottomrule
        \end{tabular}
    }
    \caption{The accuracies of silver data and clean data. Higher accuracy means lower noise level.}
    \label{tab:human_eval}
\end{table}
% The clean data detected by NLNL has much higher accuracy than the silver data.
\begin{figure}[htbp]
    \centering
    \includegraphics[width=0.49\textwidth]{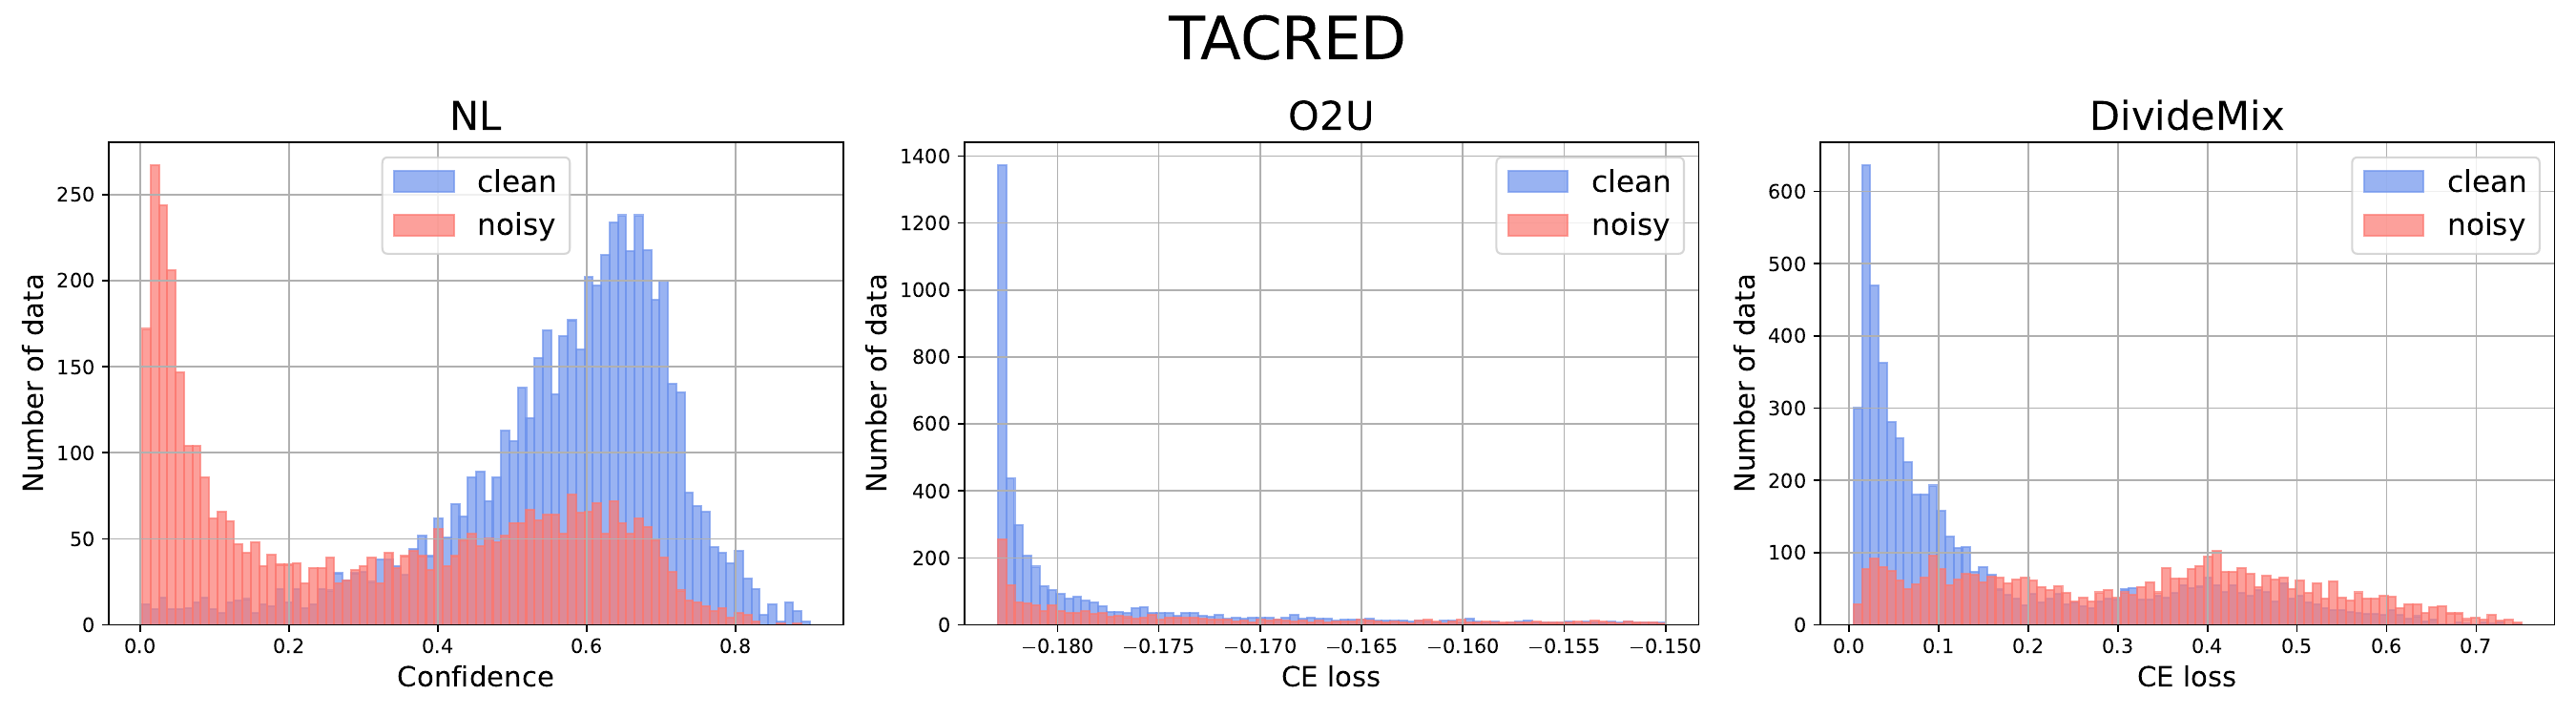}
    \includegraphics[width=0.49\textwidth]{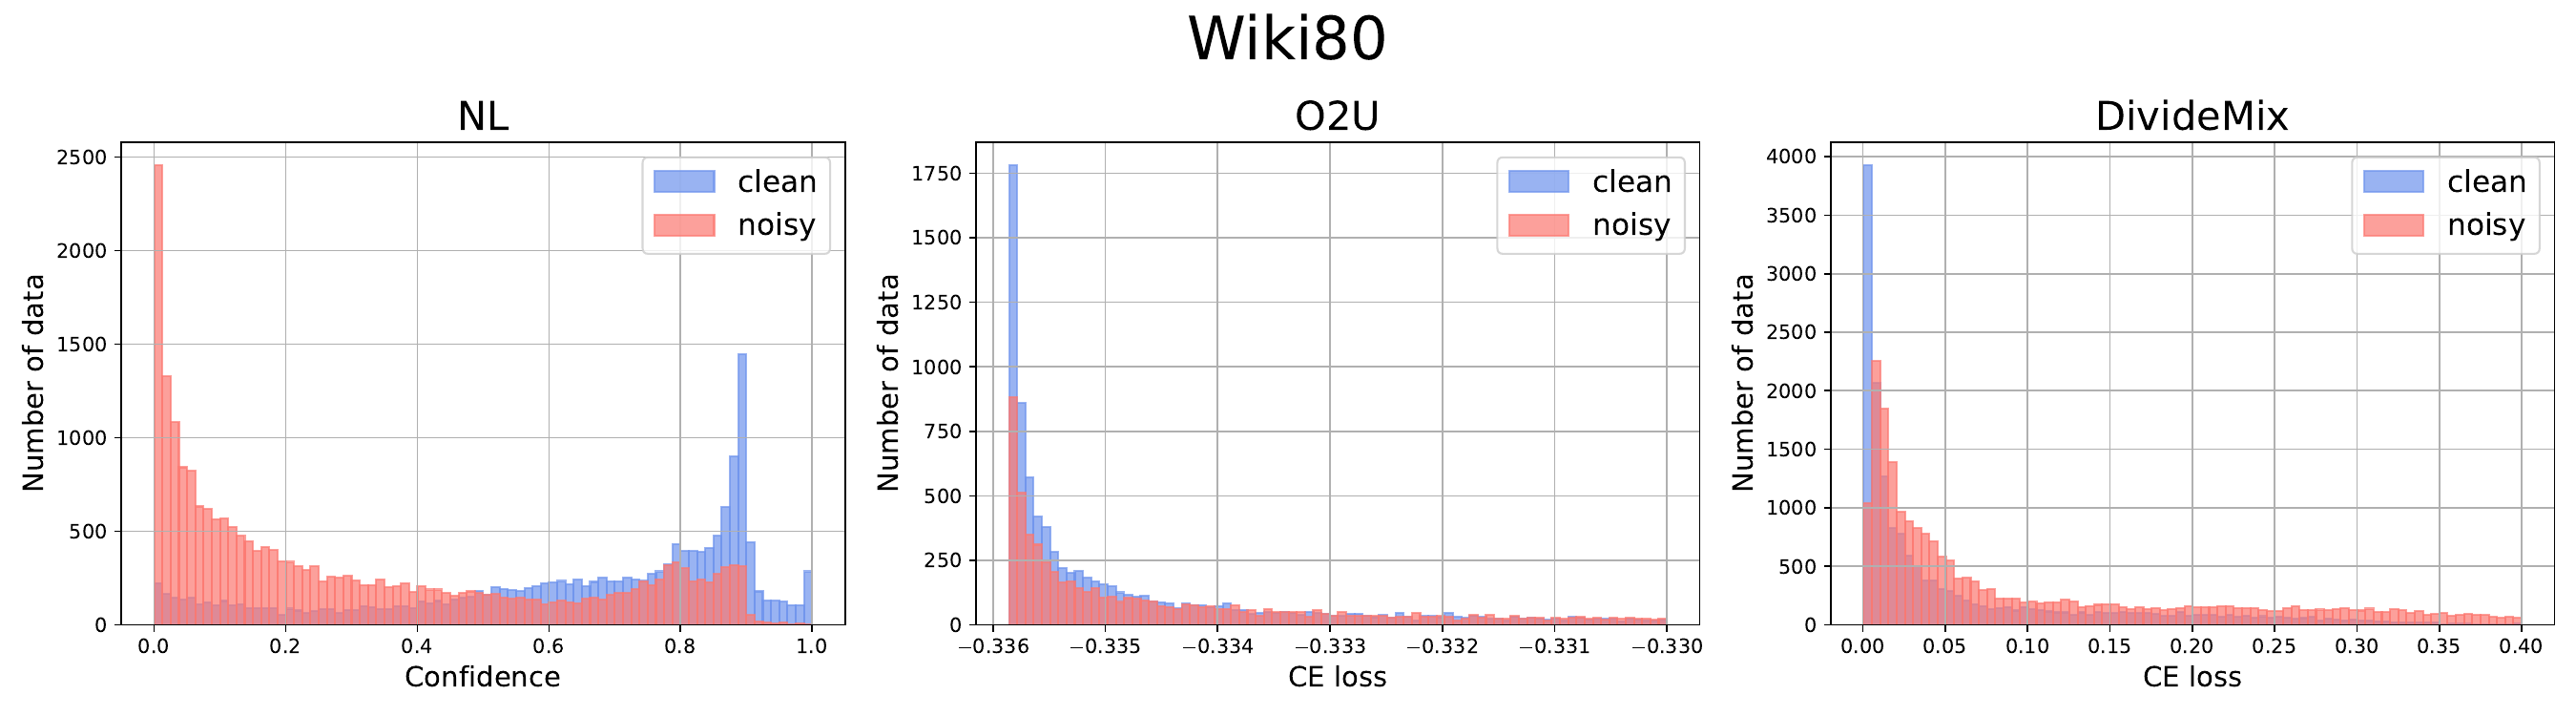}
    \caption{Histogram showing the confidence scores or losses distribution of silver standard data on TACRED and Wiki80, Blue indicates clean data, whereas red indicates noisy data. }
    \label{fig:clean_noisy}
\end{figure}

\subsection{Visualization}
\label{appendix:visualization}
We show confusion matrices of the test data on both datasets in Figure \ref{fig:confusion_matrix}. 
As shown in the figures, most of the relations are classified correctly in Clean Data Finetune method.
\subsection{Implementation Details}
\label{appendix:implement}
All of our experiments are performed on a single NVIDIA RTX 3090 GPU.
Both the Clean Data Finetune method and Class-aware Clean Data Finetune method need 1.5 hours for training.
In zero-shot and few-shot settings, the pre-trained TE model we used is  microsoft/deberta-v2-xlarge-mnli \cite{he2021deberta}. 
We also report the performance of Clean Data Finetune Method using microsoft/deberta-v2-xxlarge-mnli \cite{he2021deberta} in 
Table \ref{tab:different_models}.
The results show that xlarge model can outperform or be comparable with xxlarge model. We use the light-weighted model to save training time. 
For all the clean data detection algorithms, we adopt bert-base-uncased \cite{devlin2018bert} as the backbone model of the classifier. We use AdamW optimizer with weight decay 1e-2. 
\paragraph{\textbf{Hyper-parameters Settings.}}
As shown in Figure \ref{fig:hyperparameters_analysis} (left), for the Clean Data Finetune method, $\eta=0.05$ for TACRED and $\eta=0.07$ for Wiki80 have the best performance on 1\% development set. 
Thus we set $\eta=0.05$ for TACRED and $\eta=0.07$ for Wiki80 in the method of Clean Data Finetune. 
For Class-aware Clean Data Finetune (Dynamic) method, we do not tune $\eta$ and we use the optimal $\eta$ as the Clean Data Finetune method uses on both datasets.

As shown in Figure \ref{fig:hyperparameters_analysis} (right), we use the expansion ratios $\delta=100$ for TACRED and $\delta=200$ for Wiki80 in the method of Class-aware Clean Data Finetune (Dynamic).
\paragraph{\textbf{Clean Data Detection Module Settings.}}
1) For O2U:  In the pre-training step, the constant learning rate is 5e-6. In cyclical training, the cyclical learning rate is linearly adjusted from 5e-6 to 1e-7 in a cycle round. 
The cycle length is five epochs in a cycle round, and we adopt one cycle round.
2) For NLNL: The learning rate is 4e-7. The number of complementary labels on a single input label is the same as the classification number. We run ten epochs. 
3) For DivideMix: The sharpening temperature $T$ is 0.5, the parameter for Beta is 4, the weight for unsupervised loss is 25, and clean probability threshold is 0.5. The learning rate is 4e-7. 
\paragraph{\textbf{Finetuning Settings.}} We use 80\% of silver standard data to finetune TE model, while the remaining 20\% data serves as the development set. The learning rate is warmed up linearly to 4e-7 and then it decreases following the values of the cosine function between 4e-7 to zero. 

\begin{table}[t]
    \centering
    \resizebox{0.49\textwidth}{!}{
        \LARGE
        \begin{tabular}{ m{6cm}<{\centering} |
        m{1.1cm}<{\centering} m{1.1cm}<{\centering} m{2.8cm}<{\centering} | m{1.1cm}<{\centering} m{1.1cm}<{\centering} m{2.8cm}<{\centering} 
        }
            \toprule
              Model & \multicolumn{3}{c}{TACRED} & \multicolumn{3}{c}{Wiki80}  \\
             
              &  Pr. & Rec. & F1 & Pr. & Rec. & F1   \\
            \midrule
            \midrule
            % &&&&&&\\
          microsoft/deberta-v2-xlarge-mnli & 53.92 & 53.93 & 62.08\Large{$\pm0.89$} & 57.50 & 49.94 & 49.94\Large{$\pm0.23$} \\ 
        %   &&&&&&\\
          \midrule
        %   &&&&&&\\
          microsoft/deberta-v2-xxlarge-mmli & 48.62 &  57.23 & 59.12\Large{$\pm2.29$} & 55.44 & 50.04 & 50.04\Large{$\pm1.16$}\\ 
        %   &&&&&& \\
            \bottomrule
        \end{tabular}
    }
    \caption{F1 scores of Clean Data Finetune method on TACRED and Wiki80 using different sizes of textual entailment model.}
    % ($k = \{1,2,3\}$)
    \label{tab:different_models}
\end{table}

\begin{figure*}[t]
	\centering
	\subfigure[TACRED]{\label{fig:yelp2015head}
		\includegraphics[width=0.9\textwidth]{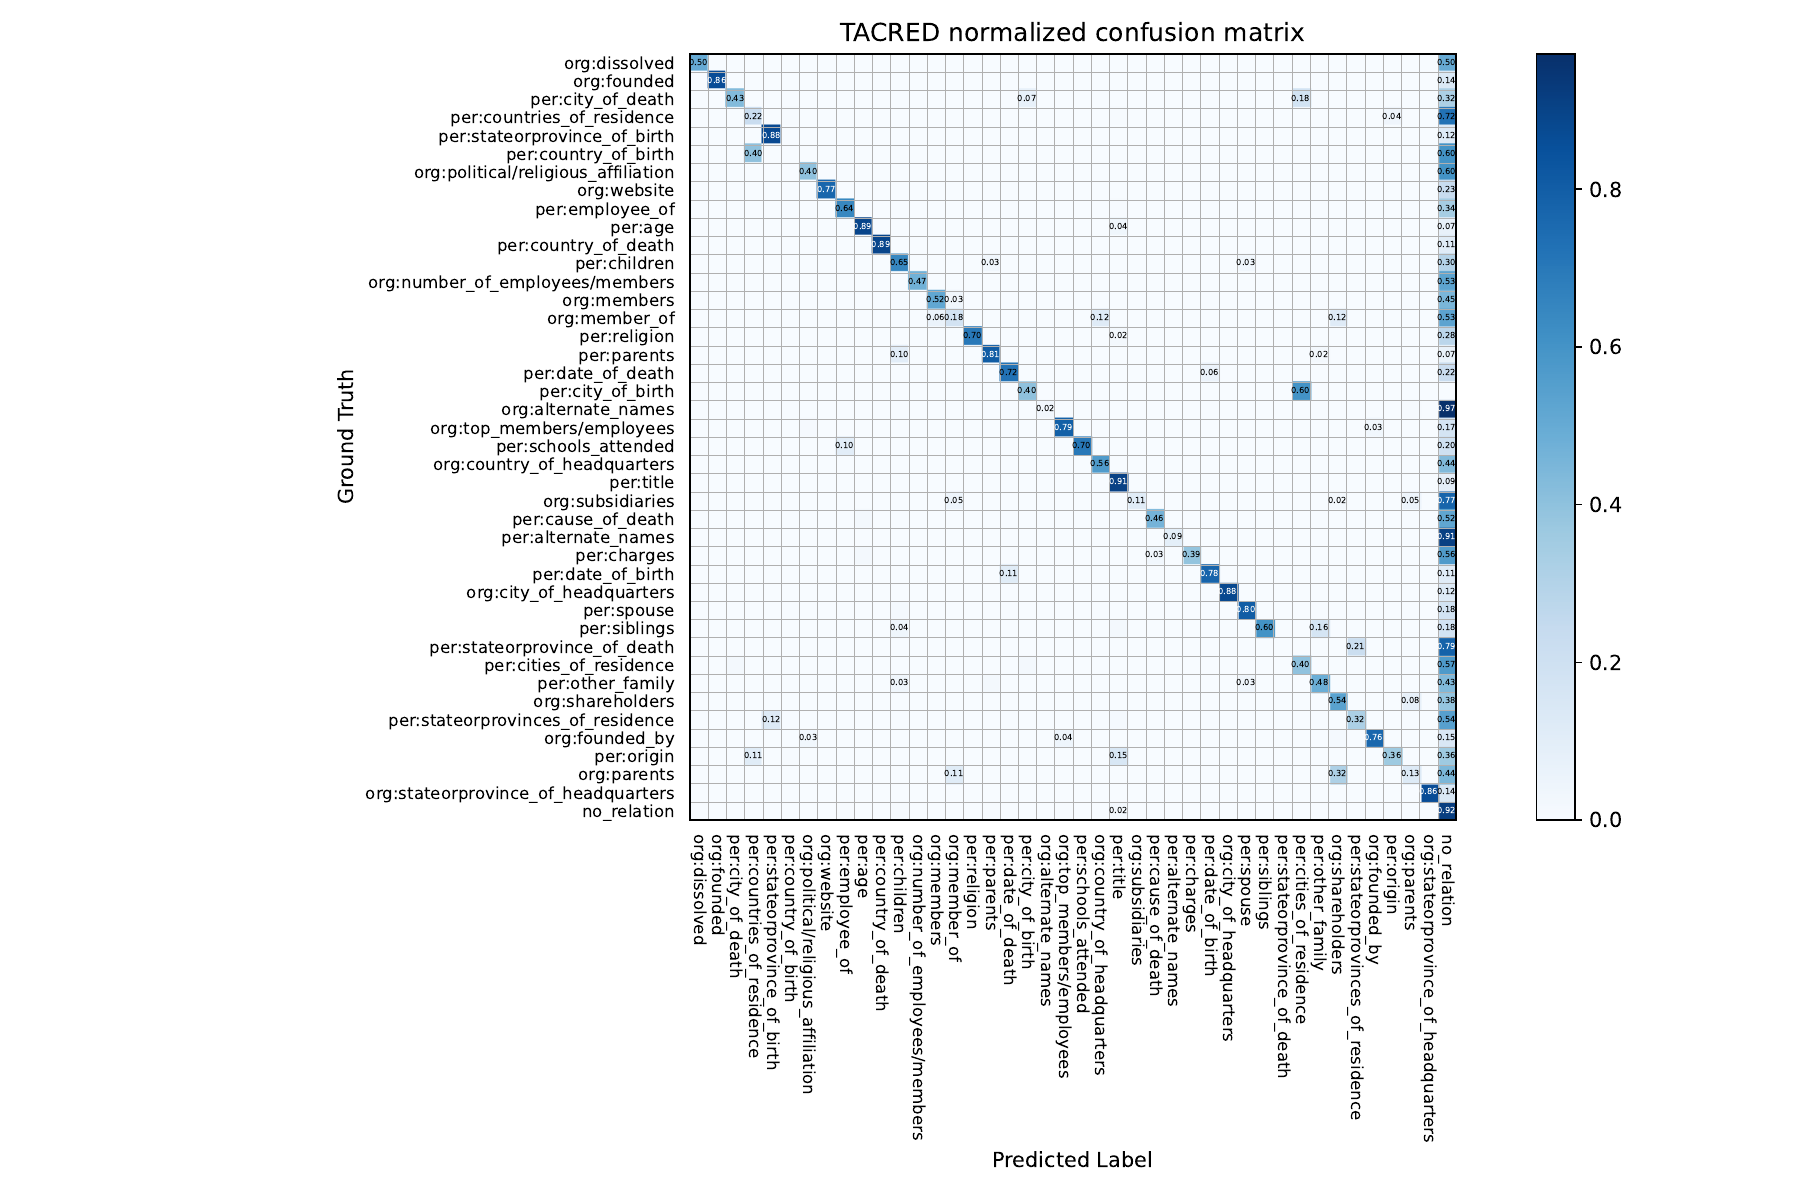}
	}
	\subfigure[Wiki80]{\label{fig:yelp2015tail}
		\includegraphics[width=0.8\textwidth]{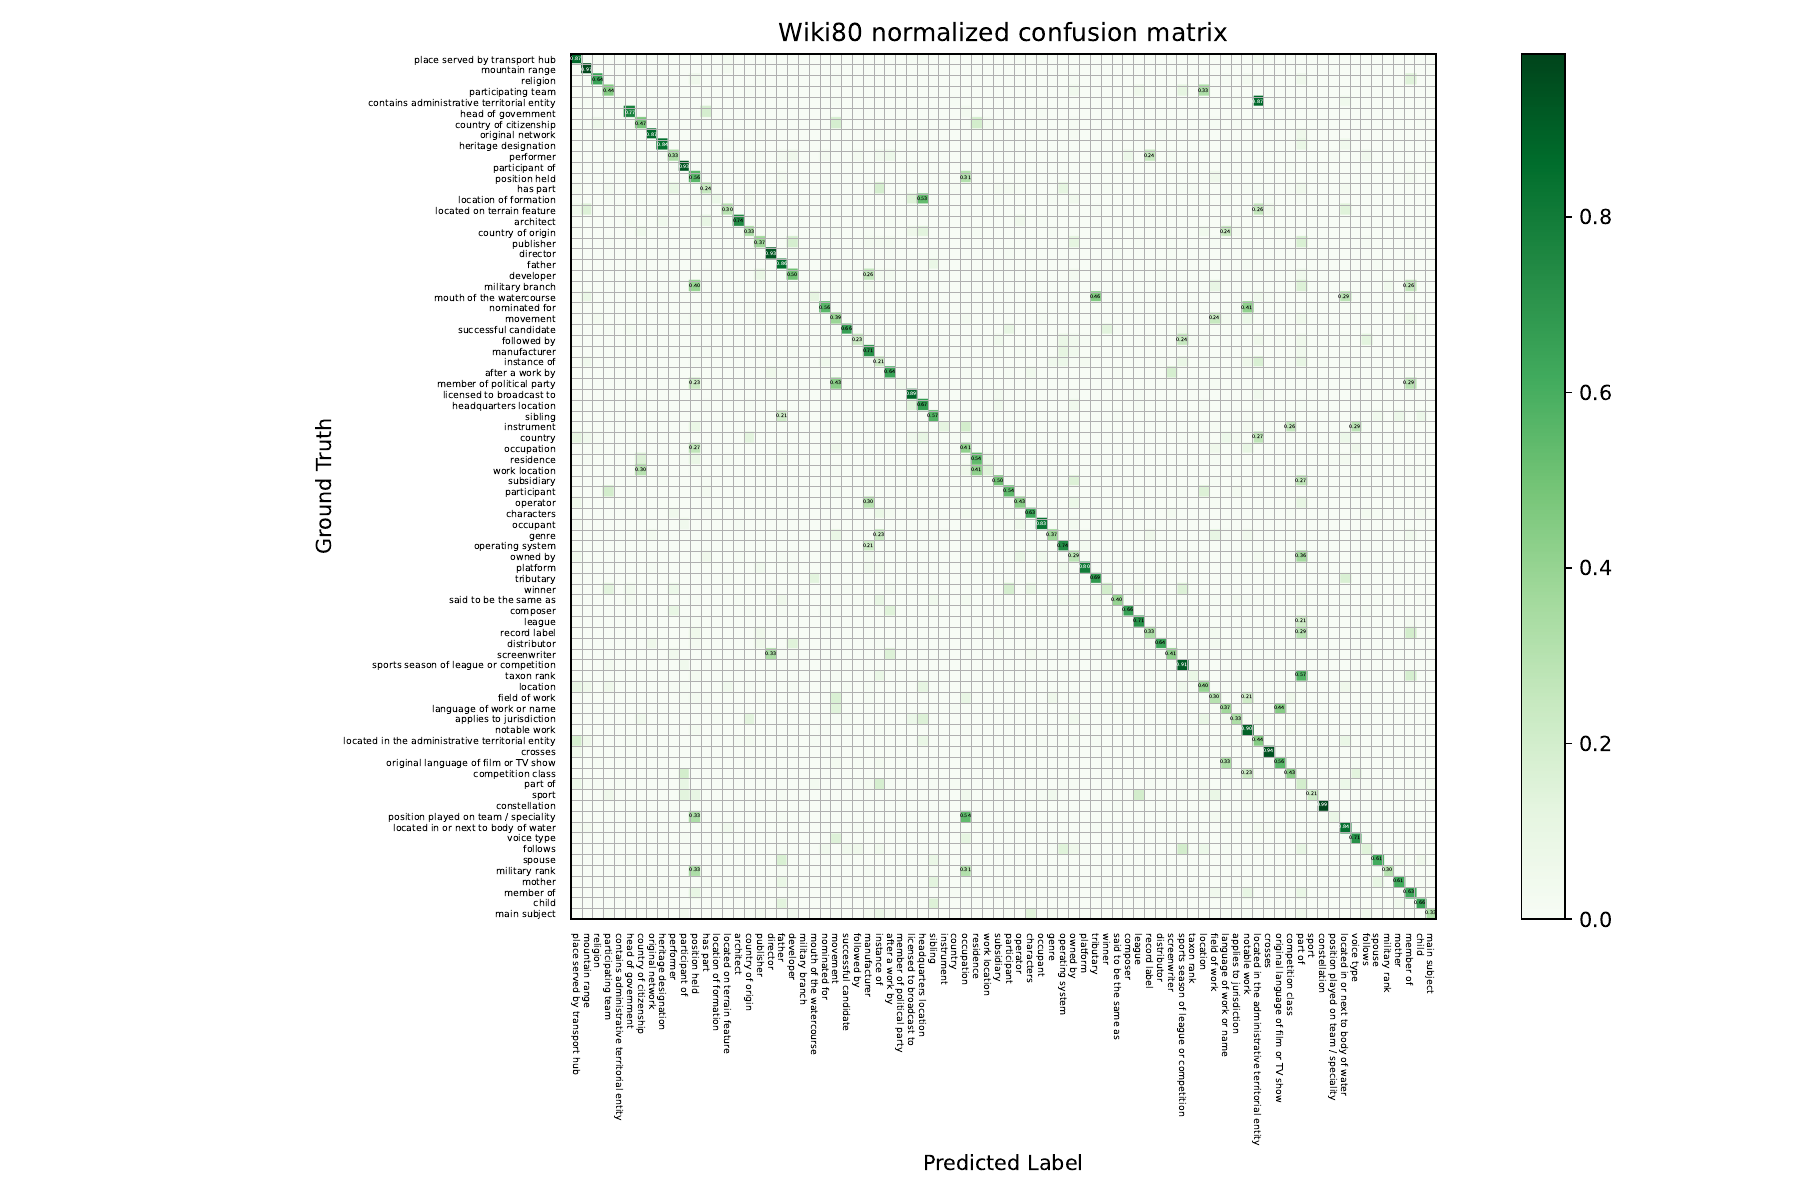}
	}
	%\vspace{-0.1in}
	\caption{ 
	    Confusion matrix (rowise normalized) of Clean Data Finetune on the test set of TACRED and Wiki80.
	}	\label{fig:confusion_matrix}
\end{figure*}

\subsection{Verbalization Templates}
\label{appendix:template}
% \revisejw{how about only reporting one dataset? there are not space left for reporting type constraints?}
% \revisezq{Unlimited pages for appendix.}
% /home/jwwang/URE/coreStandfordTagging/dataPreview.ipynb
\subsubsection{TACRED}
We show verbalization templates of all relation types on TACRED in Table \ref{TACRED_template}.
\begin{table*}[ht]
    \centering
    \resizebox{1\textwidth}{!}{
        \begin{tabular}[h]{c  c  c  c }
    \hline
    Relation & Template  & Relation & Template \\
    \hline
    
no\_relation & \makecell[c]{\{subj\} and \{obj\} are not related} & 
per:alternate\_names & \makecell[c]{\{subj\} is also known as \{obj\}}   \\\\ 
per:date\_of\_birth & \makecell[c]{\{subj\} 's birthday is on \{obj\} \\ \{subj\} was born in \{obj\}} & 
per:age & \makecell[c]{\{subj\} is \{obj\} years old}   \\\\ 
per:country\_of\_birth & \makecell[c]{\{subj\} was born in \{obj\}} & 
per:stateorprovince\_of\_birth & \makecell[c]{\{subj\} was born in \{obj\}}   \\\\ 
per:city\_of\_birth & \makecell[c]{\{subj\} was born in \{obj\}} & 
per:origin & \makecell[c]{\{obj\} is the nationality of \{subj\}}   \\\\ 
per:date\_of\_death & \makecell[c]{\{subj\} died in \{obj\}} & 
per:country\_of\_death & \makecell[c]{\{subj\} died in \{obj\}}   \\\\ 
per:stateorprovince\_of\_death & \makecell[c]{\{subj\} died in \{obj\}} & 
per:city\_of\_death & \makecell[c]{\{subj\} died in \{obj\}}   \\\\ 
per:cause\_of\_death & \makecell[c]{\{obj\} is the cause of \{subj\}'s death} & 
per:countries\_of\_residence & \makecell[c]{\{subj\} lives in \{obj\} \\ \{subj\} has a legal order to stay in \{obj\}}   \\\\ 
per:stateorprovinces\_of\_residence & \makecell[c]{\{subj\} lives in \{obj\} \\ \{subj\} has a legal order to stay in \{obj\}} & 
per:cities\_of\_residence & \makecell[c]{\{subj\} lives in \{obj\} \\ \{subj\} has a legal order to stay in \{obj\}}   \\\\ 
per:schools\_attended & \makecell[c]{\{subj\} studied in \{obj\} \\ \{subj\} graduated from \{obj\}} & 
per:title & \makecell[c]{\{subj\} is a \{obj\}}   \\\\ 
per:employee\_of & \makecell[c]{\{subj\} is member of \{obj\} \\ \{subj\} is an employee of \{obj\}} & 
per:religion & \makecell[c]{\{subj\} belongs to \{obj\} religion \\ \{obj\} is the religion of \{subj\} \\ \{subj\} believe in \{obj\}}   \\\\ 
per:spouse & \makecell[c]{\{subj\} is the spouse of \{obj\} \\ \{subj\} is the wife of \{obj\} \\ \{subj\} is the husband of \{obj\}} & 
per:parents & \makecell[c]{\{obj\} is the parent of \{subj\} \\ \{obj\} is the mother of \{subj\} \\ \{obj\} is the father of \{subj\} \\ \{subj\} is the son of \{obj\} \\ \{subj\} is the daughter of \{obj\}}   \\\\ 
per:children & \makecell[c]{\{subj\} is the parent of \{obj\} \\ \{subj\} is the mother of \{obj\} \\ \{subj\} is the father of \{obj\} \\ \{obj\} is the son of \{subj\} \\ \{obj\} is the daughter of \{subj\}} & 
per:siblings & \makecell[c]{\{subj\} and \{obj\} are siblings \\ \{subj\} is brother of \{obj\} \\ \{subj\} is sister of \{obj\}}   \\\\ 
per:other\_family & \makecell[c]{\{subj\} and \{obj\} are family \\ \{subj\} is a brother in law of \{obj\} \\ \{subj\} is a sister in law of \{obj\} \\ \{subj\} is the cousin of \{obj\} \\ \{subj\} is the uncle of \{obj\} \\ \{subj\} is the aunt of \{obj\} \\ \{subj\} is the grandparent of \{obj\} \\ \{subj\} is the grandmother of \{obj\} \\ \{subj\} is the grandson of \{obj\} \\ \{subj\} is the granddaughter of \{obj\}} & 
per:charges & \makecell[c]{\{subj\} was convicted of \{obj\} \\ \{obj\} are the charges of \{subj\}}   \\\\ 
org:alternate\_names & \makecell[c]{\{subj\} is also known as \{obj\}} & 
org:political/religious\_affiliation & \makecell[c]{\{subj\} has political affiliation with \{obj\} \\ \{subj\} has religious affiliation with \{obj\}}   \\\\ 
org:top\_members/employees & \makecell[c]{\{obj\} is a high level member of \{subj\} \\ \{obj\} is chairman of \{subj\} \\ \{obj\} is president of \{subj\} \\ \{obj\} is director of \{subj\}} & 
org:number\_of\_employees/members & \makecell[c]{\{subj\} employs nearly \{obj\} people \\ \{subj\} has about \{obj\} employees}   \\\\ 
org:members & \makecell[c]{\{obj\} is member of \{subj\} \\ \{obj\} joined \{subj\}} & 
org:member\_of & \makecell[c]{\{subj\} is member of \{obj\} \\ \{subj\} joined \{obj\}}   \\\\ 
org:subsidiaries & \makecell[c]{\{obj\} is a subsidiary of \{subj\} \\ \{obj\} is a branch of \{subj\}} & 
org:parents & \makecell[c]{\{subj\} is a subsidiary of \{obj\} \\ \{subj\} is a branch of \{obj\}}   \\\\ 
org:founded\_by & \makecell[c]{\{subj\} was founded by \{obj\} \\ \{obj\} founded \{subj\}} & 
org:founded & \makecell[c]{\{subj\} was founded in \{obj\} \\ \{subj\} was formed in \{obj\}}   \\\\ 
org:dissolved & \makecell[c]{\{subj\} existed until \{obj\} \\ \{subj\} disbanded in \{obj\} \\ \{subj\} dissolved in \{obj\}} & 
org:country\_of\_headquarters & \makecell[c]{\{subj\} has its headquarters in \{obj\} \\ \{subj\} is located in \{obj\}}   \\\\ 
org:stateorprovince\_of\_headquarters & \makecell[c]{\{subj\} has its headquarters in \{obj\} \\ \{subj\} is located in \{obj\}} & 
org:city\_of\_headquarters & \makecell[c]{\{subj\} has its headquarters in \{obj\} \\ \{subj\} is located in \{obj\}}   \\\\ 
org:shareholders & \makecell[c]{\{obj\} holds shares in \{subj\}} & 
org:website & \makecell[c]{\{obj\} is the URL of \{subj\} \\ \{obj\} is the website of \{subj\}}   \\\\ 

\hline

        \end{tabular}
    }
    \caption{Verbalization templates on TACRED.}
    \label{TACRED_template}
\end{table*}

\subsubsection{Wiki80}
We show verbalization templates of all relation types on Wiki80 in Table \ref{Wiki80_template}.
 
\begin{table*}[ht]
    \centering
    \resizebox{1\textwidth}{!}{
        \begin{tabular}[h]{c  c  c  c }
    \hline
    Relation & Template  & Relation & Template \\
    \hline
place served by transport hub & \makecell[c]{\{subj\} is the place that served by a transport hub in \{obj\}.} & 
mountain range & \makecell[c]{\{subj\} mountain range is in the \{obj\}. \\ \{subj\} mountain range is on the \{obj\}. \\ \{subj\} mountain range is part of the \{obj\}.}   \\\\ 
religion & \makecell[c]{\{obj\} is \{subj\}'s religion.} & 
participating team & \makecell[c]{\{obj\} team participated in \{subj\}. \\ \{obj\} rival participated in \{subj\}.}   \\\\ 
contains administrative territorial entity & \makecell[c]{\{obj\} place is the terrioty of \{subj\}.} & 
head of government & \makecell[c]{\{obj\} is the government head of \{subj\}.}   \\\\ 
country of citizenship & \makecell[c]{\{obj\} country does \{subj\} has a citizenship of.} & 
original network & \makecell[c]{\{obj\} is the original network of \{subj\}.}   \\\\ 
heritage designation & \makecell[c]{\{subj\} heritage designation is listed on the \{obj\}.} & 
performer & \makecell[c]{\{obj\} are performers of " \{subj\} ".}   \\\\ 
participant of & \makecell[c]{\{subj\} participated in \{obj\}. \\ \{obj\} event did \{subj\} participate in.} & 
position held & \makecell[c]{\{obj\} position is held by \{subj\}.}   \\\\ 
has part & \makecell[c]{\{subj\} does \{obj\} belong to.} & 
location of formation & \makecell[c]{\{obj\} is \{subj\} formed.}   \\\\ 
located on terrain feature & \makecell[c]{\{obj\} is the terrain feature \{subj\} located in.} & 
architect & \makecell[c]{\{obj\} is the architect of \{subj\}.}   \\\\ 
country of origin & \makecell[c]{\{obj\} is \{subj\}'s country of origin.} & 
publisher & \makecell[c]{\{obj\} is the publisher of " \{subj\} ".}   \\\\ 
director & \makecell[c]{\{obj\} is the director of " \{subj\} ".} & 
father & \makecell[c]{\{obj\} is \{subj\}'s father.}   \\\\ 
developer & \makecell[c]{\{obj\} is the developer of " \{subj\} ".} & 
military branch & \makecell[c]{\{obj\} military branch does \{subj\} work for.}   \\\\ 
mouth of the watercourse & \makecell[c]{\{subj\} is the mouth of the watercourse \{obj\}.} & 
nominated for & \makecell[c]{\{obj\} are " \{subj\} " nominated for. \\ \{subj\} is the nominee of \{obj\}.}   \\\\ 
movement & \makecell[c]{\{obj\} is movement of \{subj\}.} & 
successful candidate & \makecell[c]{\{obj\} is the successful candidate of \{subj\}.}   \\\\ 
followed by & \makecell[c]{\{subj\} is before " \{obj\} ". \\ \{subj\} is followed by " \{obj\} ".} & 
manufacturer & \makecell[c]{\{obj\} is the manufacturer of \{subj\}.}   \\\\ 
instance of & \makecell[c]{\{subj\} is an instance of \{obj\}. \\ \{obj\} is the \{subj\}.} & 
after a work by & \makecell[c]{\{subj\} is created by " \{obj\} ". \\ \{subj\} is based on " \{obj\} ".}   \\\\ 
member of political party & \makecell[c]{\{obj\} political party does \{subj\} belong to.} & 
licensed to broadcast to & \makecell[c]{\{subj\} is licensed to \{obj\}.}   \\\\ 
headquarters location & \makecell[c]{\{obj\} is the headquarter of \{subj\}.} & 
sibling & \makecell[c]{\{obj\} are \{subj\}'siblings. \\ \{subj\} are \{obj\}'s siblings.}   \\\\ 
instrument & \makecell[c]{\{obj\} instruments does \{subj\} play.} & 
country & \makecell[c]{\{obj\} country does \{subj\} belong to.}   \\\\ 
occupation & \makecell[c]{\{obj\} is \{subj\}'s occupation.} & 
residence & \makecell[c]{\{obj\} does \{subj\} live in.}   \\\\ 
work location & \makecell[c]{\{obj\} does \{subj\} work in.} & 
subsidiary & \makecell[c]{\{obj\} organization is the subsidiary of \{subj\}.}   \\\\ 
participant & \makecell[c]{\{obj\} are participants of \{subj\}.} & 
operator & \makecell[c]{\{obj\} are operators of \{subj\}.}   \\\\ 
characters & \makecell[c]{\{obj\} are the characters of \{subj\}.} & 
occupant & \makecell[c]{\{obj\} teams are occupants of \{subj\}.}   \\\\ 
genre & \makecell[c]{\{obj\} is the genre of " \{subj\} ".} & 
operating system & \makecell[c]{\{obj\} are operating systems of \{subj\}.}   \\\\ 
owned by & \makecell[c]{\{obj\} own \{subj\}.} & 
platform & \makecell[c]{\{subj\} are platforms of \{obj\}.}   \\\\ 
tributary & \makecell[c]{\{obj\} are tributaries of \{subj\}.} & 
winner & \makecell[c]{\{obj\} are the winners of \{subj\}.}   \\\\ 
said to be the same as & \makecell[c]{\{obj\} are said to be the same as \{subj\}.} & 
composer & \makecell[c]{\{obj\} are composers of \{subj\}.}   \\\\ 
league & \makecell[c]{\{obj\} is the league of \{subj\}.} & 
record label & \makecell[c]{\{obj\} is the record label of \{subj\}.}   \\\\ 
distributor & \makecell[c]{\{obj\} are distributors of \{subj\}.} & 
screenwriter & \makecell[c]{\{obj\} are screenwriters of \{subj\}.}   \\\\ 
sports season of league or competition & \makecell[c]{\{subj\} seasons of \{obj\} are mentioned.} & 
taxon rank & \makecell[c]{\{obj\} is taxon rank of \{subj\}.}   \\\\ 
location & \makecell[c]{\{obj\} did \{subj\} held.} & 
field of work & \makecell[c]{\{obj\} are \{subj\}'s fields of work.}   \\\\ 
language of work or name & \makecell[c]{\{obj\} is the language of the work " \{subj\} ". \\ \{obj\} is the language of the name " \{subj\} ".} & 
applies to jurisdiction & \makecell[c]{\{obj\} is the jurisdiction of \{subj\} applied to.}   \\\\ 
notable work & \makecell[c]{\{obj\} are notable works of \{subj\}.} & 
located in the administrative territorial entity & \makecell[c]{\{obj\} is the administrative territorial entity \{subj\} located in.}   \\\\ 
crosses & \makecell[c]{\{subj\} cross \{obj\}.} & 
original language of film or TV show & \makecell[c]{\{obj\} is the original language of the film " \{subj\} ". \\ \{obj\} is the original language of the TV show " \{subj\} ".}   \\\\ 
competition class & \makecell[c]{\{obj\} is the competition class of \{subj\}.} & 
part of & \makecell[c]{\{subj\} is a part of \{obj\}.}   \\\\ 
sport & \makecell[c]{\{obj\} sports does \{subj\} play.} & 
constellation & \makecell[c]{\{subj\} are in the constellation of " \{obj\} ".}   \\\\ 
position played on team / speciality & \makecell[c]{\{obj\} position does \{subj\} play on the team.} & 
located in or next to body of water & \makecell[c]{\{obj\} body of water is \{subj\} located in.}   \\\\ 
voice type & \makecell[c]{\{obj\} is the voice type of \{subj\}.} & 
follows & \makecell[c]{\{subj\} is after " \{obj\} ". \\ \{subj\} follows " \{obj\} ".}   \\\\ 
spouse & \makecell[c]{\{obj\} is \{subj\}'s spouse.} & 
military rank & \makecell[c]{\{obj\} is the military rank of \{subj\}.}   \\\\ 
mother & \makecell[c]{\{obj\} is \{subj\}'s mother.} & 
member of & \makecell[c]{\{subj\} is a member of \{obj\}.}   \\\\ 
child & \makecell[c]{\{obj\} are \{subj\}'s children.} & 
main subject & \makecell[c]{\{obj\} is the main subject of " \{subj\} ".}   \\\\

\hline

        \end{tabular}
    }
    \caption{Verbalization templates on Wiki80.}
    \label{Wiki80_template}
\end{table*}

\subsection{Entity Type Constraints}
\label{appendix:constraint}
\subsubsection{TACRED}
We present the entity type constraints of relation types on TACRED in Table \ref{Tacred_constraints}. 
% The constraints are different from that of LaVeEntail. We delete the constraints which leak the information of the ground truth. 
% For example, there is only one relation type that has the constraint where the subject entity type is \texttt{PERSON} and the object entity type is \texttt{TITLE}. 
% The sentence that satisfies this constraint has a very large probability to be inferred as \texttt{per:title} relation because other relations are ruled out. 
% \citep{tran2020revisiting} showed that entity types are a strong inductive bias. But in LaVeEntail, the inductive bias is not learned by the algorithm itself but by manually designed type constraints. It leads to artificially inflated performance, so we deleted those type constraints.
\begin{table*}[ht]
    \centering
    \resizebox{1\textwidth}{!}{
        \begin{tabular}[h]{c  c  c  c }
    \hline
    Relation & Constraint  & Relation & Constraint \\
    \hline
    per:alternate\_names & \makecell[c]{PERSON:PERSON} & 
per:date\_of\_birth & \makecell[c]{PERSON:DATE}   \\\\ 

per:age & \makecell[c]{PERSON:TITLE , PERSON:CITY , PERSON:STATE\_OR\_PROVINCE \\ PERSON:ORGANIZATION , PERSON:RELIGION , PERSON:DURATION \\ PERSON:NUMBER , PERSON:LOCATION , PERSON:DATE \\ PERSON:NATIONALITY , PERSON:IDEOLOGY , PERSON:PERSON \\ PERSON:MISC , PERSON:COUNTRY , PERSON:CAUSE\_OF\_DEATH \\ PERSON:URL , PERSON:CRIMINAL\_CHARGE}  & 
per:country\_of\_birth & \makecell[c]{PERSON:COUNTRY}   \\\\

per:stateorprovince\_of\_birth & \makecell[c]{PERSON:STATE\_OR\_PROVINCE} & 
per:city\_of\_birth & \makecell[c]{PERSON:CITY}   \\\\ 

per:origin & \makecell[c]{PERSON:NATIONALITY , PERSON:COUNTRY , PERSON:LOCATION}  &
per:date\_of\_death & \makecell[c]{PERSON:DATE}   \\\\ 

per:country\_of\_death & \makecell[c]{PERSON:COUNTRY} & 
per:stateorprovince\_of\_death & \makecell[c]{PERSON:STATE\_OR\_PROVICE}   \\\\ 

per:city\_of\_death & \makecell[c]{PERSON:CITY} & 
per:cause\_of\_death & \makecell[c]{PERSON:TITLE , PERSON:CITY , PERSON:STATE\_OR\_PROVINCE \\ PERSON:ORGANIZATION , PERSON:RELIGION , PERSON:DURATION \\ PERSON:NUMBER , PERSON:LOCATION , PERSON:DATE \\ PERSON:NATIONALITY , PERSON:IDEOLOGY , PERSON:PERSON \\ PERSON:MISC , PERSON:COUNTRY , PERSON:CAUSE\_OF\_DEATH \\ PERSON:URL , PERSON:CRIMINAL\_CHARGE}   \\\\ 

per:countries\_of\_residence & \makecell[c]{PERSON:COUNTRY , PERSON:NATIONALITY} & 
per:stateorprovinces\_of\_residence & \makecell[c]{PERSON:STATE\_OR\_PROVINCE}   \\\\ 

per:cities\_of\_residence & \makecell[c]{PERSON:CITY} & 
per:schools\_attended & \makecell[c]{PERSON:ORGANIZATION}   \\\\ 

per:title & \makecell[c]{PERSON:TITLE , PERSON:CITY , PERSON:STATE\_OR\_PROVINCE \\ PERSON:ORGANIZATION , PERSON:RELIGION , PERSON:DURATION \\ PERSON:NUMBER , PERSON:LOCATION , PERSON:DATE \\ PERSON:NATIONALITY , PERSON:IDEOLOGY , PERSON:PERSON \\ PERSON:MISC , PERSON:COUNTRY , PERSON:CAUSE\_OF\_DEATH \\ PERSON:URL , PERSON:CRIMINAL\_CHARGE}  &
per:employee\_of & \makecell[c]{PERSON:ORGANIZATION}   \\\\ 

per:religion & \makecell[c]{PERSON:TITLE , PERSON:CITY , PERSON:STATE\_OR\_PROVINCE \\ PERSON:ORGANIZATION , PERSON:RELIGION , PERSON:DURATION \\ PERSON:NUMBER , PERSON:LOCATION , PERSON:DATE \\ PERSON:NATIONALITY , PERSON:IDEOLOGY , PERSON:PERSON \\ PERSON:MISC , PERSON:COUNTRY , PERSON:CAUSE\_OF\_DEATH \\ PERSON:URL , PERSON:CRIMINAL\_CHARGE}  &
per:spouse & \makecell[c]{PERSON:PERSON}   \\\\ 

per:parents & \makecell[c]{PERSON:PERSON} & 
per:children & \makecell[c]{PERSON:PERSON}   \\\\ 

per:siblings & \makecell[c]{PERSON:PERSON} & 
per:other\_family & \makecell[c]{PERSON:PERSON}   \\\\ 

per:charges & \makecell[c]{PERSON:TITLE , PERSON:CITY , PERSON:STATE\_OR\_PROVINCE \\ PERSON:ORGANIZATION , PERSON:RELIGION , PERSON:DURATION \\ PERSON:NUMBER , PERSON:LOCATION , PERSON:DATE \\ PERSON:NATIONALITY , PERSON:IDEOLOGY , PERSON:PERSON \\ PERSON:MISC , PERSON:COUNTRY , PERSON:CAUSE\_OF\_DEATH \\ PERSON:URL , PERSON:CRIMINAL\_CHARGE}  & 
org:alternate\_names & \makecell[c]{ORGANIZATION:ORGANIZATION}   \\\\ 

org:political/religious\_affiliation & \makecell[c]{ORGANIZATION:TITLE , ORGANIZATION:CITY , ORGANIZATION:STATE\_OR\_PROVINCE \\ ORGANIZATION:ORGANIZATION , ORGANIZATION:RELIGION , ORGANIZATION:DURATION \\ ORGANIZATION:NUMBER , ORGANIZATION:LOCATION , ORGANIZATION:DATE \\ ORGANIZATION:NATIONALITY , ORGANIZATION:IDEOLOGY , ORGANIZATION:PERSON \\ ORGANIZATION:MISC , ORGANIZATION:COUNTRY , ORGANIZATION:CAUSE\_OF\_DEATH \\ ORGANIZATION:URL , ORGANIZATION:CRIMINAL\_CHARGE}   &
org:top\_members/employees & \makecell[c]{ORGANIZATION:PERSON}   \\\\ 

org:number\_of\_employees/members & \makecell[c]{ORGANIZATION:TITLE , ORGANIZATION:CITY , ORGANIZATION:STATE\_OR\_PROVINCE \\ ORGANIZATION:ORGANIZATION , ORGANIZATION:RELIGION , ORGANIZATION:DURATION \\ ORGANIZATION:NUMBER , ORGANIZATION:LOCATION , ORGANIZATION:DATE \\ ORGANIZATION:NATIONALITY , ORGANIZATION:IDEOLOGY , ORGANIZATION:PERSON \\ ORGANIZATION:MISC , ORGANIZATION:COUNTRY , ORGANIZATION:CAUSE\_OF\_DEATH \\ ORGANIZATION:URL , ORGANIZATION:CRIMINAL\_CHARGE}   &
org:members & \makecell[c]{ORGANIZATION:ORGANIZATION}   \\\\ 

org:member\_of & \makecell[c]{ORGANIZATION:ORGANIZATION , ORGANIZATION:COUNTRY , ORGANIZATION:LOCATION \\ ORGANIZATION:STATE\_OR\_PROVINCE} & 
org:subsidiaries & \makecell[c]{ORGANIZATION:ORGANIZATION}   \\\\

org:parents & \makecell[c]{ORGANIZATION:ORGANIZATION} & 
org:founded\_by & \makecell[c]{ORGANIZATION:PERSON}   \\\\ 

org:founded & \makecell[c]{ORGANIZATION:DATE} & 
org:dissolved & \makecell[c]{ORGANIZATION:DATE}   \\\\ 

org:country\_of\_headquarters & \makecell[c]{ORGANIZATION:COUNTRY} & 
org:stateorprovince\_of\_headquarters & \makecell[c]{ORGANIZATION:STATE\_OR\_PROVINCE}   \\\\ 

org:city\_of\_headquarters & \makecell[c]{ORGANIZATION:CITY} & 
org:shareholders & \makecell[c]{ORGANIZATION:PERSON , ORGANIZATION:ORGANIZATION} \\\\

org:website & \makecell[c]{ORGANIZATION:TITLE , ORGANIZATION:CITY , ORGANIZATION:STATE\_OR\_PROVINCE \\ ORGANIZATION:ORGANIZATION , ORGANIZATION:RELIGION , ORGANIZATION:DURATION \\ ORGANIZATION:NUMBER , ORGANIZATION:LOCATION , ORGANIZATION:DATE \\ ORGANIZATION:NATIONALITY , ORGANIZATION:IDEOLOGY , ORGANIZATION:PERSON \\ ORGANIZATION:MISC , ORGANIZATION:COUNTRY , ORGANIZATION:CAUSE\_OF\_DEATH \\ ORGANIZATION:URL , ORGANIZATION:CRIMINAL\_CHARGE} & &  \\\\ 

    \hline

        \end{tabular}
    }
    \caption{Entity type constraints on TACRED.}
    \label{Tacred_constraints}
\end{table*}

\subsubsection{Wiki80}
We present the entity type constraints of relation types on Wiki80 in Table \ref{Wiki80_constraints}. 

\begin{table*}[ht]
    \centering
    \resizebox{1\textwidth}{!}{
        \begin{tabular}[h]{c  c  c  c }
    \hline
    Relation & Constraint  & Relation & Constraint \\
    \hline
place served by transport hub & \makecell[c]{FAC:GPE} & 
mountain range & \makecell[c]{MOUNTAIN:MOUNTAIN , MOUNTAIN:GLACIER , GLACIER:MOUNTAIN \\ GLACIER:GLACIER} \\\\
religion & \makecell[c]{LOC:NORP , GPE:NORP , ORG:NORP} &  % ok right here
participating team & \makecell[c]{EVENT:GPE}  \\\\

contains administrative territorial entity & \makecell[c]{GPE:GPE} & 
head of government & \makecell[c]{GPE:PERSON}   \\\\

country of citizenship & \makecell[c]{PERSON:GPE} & 
original network & \makecell[c]{BROADCASTER:ORG , NETWORK:ORG} \\\\

heritage designation & \makecell[c]{WORK\_OF\_ART:LOC} & 
performer & \makecell[c]{WORK\_OF\_ART:PERSON}   \\\\ 

participant of & \makecell[c]{PERSON:EVENT} & 
position held & \makecell[c]{LOC:EVENT}   \\\\ 

has part & \makecell[c]{ORG:PERSON} & 
location of formation & \makecell[c]{ORG:GPE}   \\\\ 

located on terrain feature & \makecell[c]{GPE:LOC , GPE:GPE} & 
architect & \makecell[c]{FAC:PERSON}   \\\\ 

country of origin & \makecell[c]{PERSON:GPE} & 
publisher & \makecell[c]{WORK\_OF\_ART:ORG}   \\\\ 

director & \makecell[c]{WORK\_OF\_ART:PERSON} & 
father & \makecell[c]{PERSON:PERSON}   \\\\ 

developer & \makecell[c]{GAME:ORG , SEQUEL:ORG , WEBSITE:ORG}   &
military branch & \makecell[c]{PERSON:ORG}   \\\\ 

mouth of the watercourse & \makecell[c]{RIVER:RIVER , RIVER:LAKE , RIVER:STREAM \\ RIVER:TRIBUTARY , LAKE:RIVER , LAKE:LAKE \\ LAKE:STREAM , LAKE:TRIBUTARY , STREAM:RIVER \\ STREAM:LAKE , STREAM:STREAM , STREAM:TRIBUTARY \\ TRIBUTARY:RIVER , TRIBUTARY:LAKE , TRIBUTARY:STREAM \\ TRIBUTARY:TRIBUTARY} & 
nominated for & \makecell[c]{WORK\_OF\_ART:WORK\_OF\_ART}   \\\\ 

movement & \makecell[c]{PERSON:NORP , PERSON:ORG} & 
successful candidate & \makecell[c]{DATE:PERSON}   \\\\ 

followed by & \makecell[c]{WORK\_OF\_ART:WORK\_OF\_ART} & 
manufacturer & \makecell[c]{MODEL:ORG}   \\\\ 

instance of & \makecell[c]{DATE:EVENT} & 
after a work by & \makecell[c]{WORK\_OF\_ART:WORK\_OF\_ART , WORK\_OF\_ART:PERSON} \\\\

member of political party & \makecell[c]{PERSON:POLITICAL PARTY} & 
licensed to broadcast to & \makecell[c]{ORG:GPE}   \\\\ 

headquarters location & \makecell[c]{COMPANY:GPE , CONGLOMERATE:GPE , SUBSIDIARY:GPE}  & 
sibling & \makecell[c]{PERSON:PERSON}   \\\\ 

instrument & \makecell[c]{PERSON:FAC} & 
country & \makecell[c]{PERSON:ORG , PERSON:GPE} \\\\

occupation & \makecell[c]{PERSON:PERSON} & 
residence & \makecell[c]{PERSON:GPE}   \\\\ 

work location & \makecell[c]{PERSON:GPE} & 
subsidiary & \makecell[c]{ORG:ORG}   \\\\ 

participant & \makecell[c]{EVENT:PERSON} & 
operator & \makecell[c]{PRODUCT:PERSON}   \\\\ 

characters & \makecell[c]{PERSON:PERSON} & 
occupant & \makecell[c]{FAC:ORG}   \\\\

\hline

        \end{tabular}
    }
    
    \caption{Entity type constraints on Wiki80.}
    \label{Wiki80_constraints}
\end{table*}
